# Supplementary material for: Biexciton as a Feshbach resonance and Bose-Einstein condensation of paraexcitons in Cu$_{2}$O
Source: arXiv:1802.00234 source file (2018-02-01)
Supplement: Supplementary file 1 [file SI2017.pdf]

# Supplementary information

To derive equation (8), we use the function of the exchange exciton-exciton interaction in the momentum space. It is a sum of functionals of four $1s$ hydrogenlike function with different vector-variables[22,25]

$$
\begin{aligned}
U^{ex}(\mathbf{k},\mathbf{q}) \;=\; & \frac{1}{V^2}\sum_{\mathbf{p}_1,\mathbf{p}_2}\{-U_{cl}(\mathbf{p}_2)\,\mathcal{F}^*(\mathbf{p}_1)\mathcal{F}(\mathbf{p}_1-\beta\mathbf{q})\mathcal{F}^*(\mathbf{p}_1-\mathbf{p}_2-\alpha\mathbf{k}-\mathbf{q})\mathcal{F}(\mathbf{p}_1-\mathbf{p}_2-\alpha\mathbf{k}-\alpha\mathbf{q}) \\
& +2U_{cl}(\mathbf{p}_2)\,\mathcal{F}^*(\mathbf{p}_1)\mathcal{F}(\mathbf{p}_1-\mathbf{p}_2+\alpha\mathbf{q})\mathcal{F}^*(\mathbf{p}_1-\mathbf{p}_2+\beta\mathbf{k}+\mathbf{q})\mathcal{F}(\mathbf{p}_1-\mathbf{p}_2+\beta\mathbf{k}+\beta\mathbf{q}) \\
& -U_{cl}(\mathbf{p}_2)\,\mathcal{F}^*(\mathbf{p}_1)\mathcal{F}(\mathbf{p}_1+\alpha\mathbf{q})\mathcal{F}^*(\mathbf{p}_1-\mathbf{p}_2+\beta\mathbf{k}+\mathbf{q})\mathcal{F}(\mathbf{p}_1-\mathbf{p}_2+\beta\mathbf{k}+\beta\mathbf{q})\}\,, \qquad (1)
\end{aligned}
$$

where the first, second, and third terms in braces stand for contributions of the electron-electron, electron-hole and hole-hole exchange, respectively. In the place of the Coulomb potential $U_{cl}$ and exciton envelope functions $\mathcal{F}$ we insert their Fourier transformations by definition,

$$
U_{cl}(\mathbf{p}) = \int d^3r\,\exp[-i\mathbf{pr}]\frac{e^2}{\epsilon r}, \quad \mathcal{F}(\mathbf{p}) = \int d^3r\,f(r)\exp[-i\mathbf{pr}], \qquad (2)
$$

where $e$ is the elementary charge, $\epsilon$ – the dielectric constant of $Cu_2O$ and $f(r)=\exp[-r/a_x]/\left(\pi a_x^3\right)^{1/2}$ – the $1s$ hydrogenlike function in the real space. Taking into account the relation $e^2/\epsilon = 2E_b a_x$ and orthonormalization of plane waves

$$
\frac{1}{V}\sum_{\mathbf{p}}\exp[i\mathbf{p}(\mathbf{r}_1-\mathbf{r}_2) = \delta(\mathbf{r}_1-\mathbf{r}_2), \qquad (3)
$$

we obtain $U^{ex}$ in the following form

$$
\begin{aligned}
U^{ex}(\mathbf{k},\mathbf{q}) \;=\; & 2E_b\left\{\int d^3r\,\exp[i(\alpha\mathbf{k}+\mathbf{q})\mathbf{r}]\int d^3r_1\,\exp[i\beta\mathbf{q}\mathbf{r}_1]f(r_1)\,f(|\mathbf{r}_1+\mathbf{r}|)\left[-\frac{a_x}{r}+2\frac{a_x}{|\mathbf{r}_1+\mathbf{r}|}\right]\right. \\
& \times\int d^3r_2\,\exp[-i\beta\mathbf{q}\mathbf{r}_2]f(r_2)\,f(|\mathbf{r}_2+\mathbf{r}|) \\
& -\int d^3r\exp[-i\alpha\mathbf{q}\mathbf{r}]\int d^3r_1d^3r_2\exp[i\beta(\mathbf{q}+\mathbf{k})(\mathbf{r}_1-\mathbf{r}_2)] \\
& \left.\times f(|\mathbf{r}_1+\mathbf{r}/2|)\,f(|\mathbf{r}_1-\mathbf{r}/2|)f(|\mathbf{r}_2+\mathbf{r}/2|)\,f(|\mathbf{r}_2-\mathbf{r}/2|)\frac{a_x}{|\mathbf{r}_1-\mathbf{r}_2|}\right\} \qquad (4)
\end{aligned}
$$

where a few transformations have been made to the hole-hole exchange interaction term to give it the form of the last term in braces. As can be seen, the nonlocality of $U^{ex}$ is connected with the oscillating exponent in the integrand of inner integrals over $\mathbf{r}_1$ and $\mathbf{r}_2$, which approaches unity when $\beta \to 0$. In this limit, the nonlocality of $U^{ex}$ disappears and

$$
\frac{1}{V}_{\mathbf{q}}U^{ex}(2\mathbf{s},\mathbf{q})\psi(\mathbf{s}+\mathbf{q}) = \int d^3r\exp[i\mathbf{sr}]\,\mathcal{U}_0(r)\,\psi(r),
$$

where except for the sign $\mathcal{U}_0(r)$ coincides with the exchange energy $J$ in Heitler-London theory of the hydrogen molecule,[29]

$$
\begin{aligned}
\mathcal{U}_0(r) &= 2E_b\left\{-\frac{a_x}{r}\left[\int d^3r_1\, f(r_1)\, f(|\mathbf{r}_1+\mathbf{r}|)\right]^2\right.\\
&+2\int d^3r_1\, f(r_1) f(|\mathbf{r}_1+\mathbf{r}|)\frac{a_x}{|\mathbf{r}_1+\mathbf{r}|}\int d^3r_2\, f(r_2)\, f(|\mathbf{r}_2+\mathbf{r}|)\\
&\left.-\int d^3r_1 d^3r_2 f(|\mathbf{r}_1+\mathbf{r}/2|)\, f(|\mathbf{r}_1-\mathbf{r}/2|) f(|\mathbf{r}_2+\mathbf{r}/2|)\, f(|\mathbf{r}_2-\mathbf{r}/2|)\frac{a_x}{|\mathbf{r}_1-\mathbf{r}_2|}\right\}\\
&\equiv -I_{ee}(r)+2\, I_{eh}(r)-I_{hh}(r).
\end{aligned}
\tag{5}
$$

Taking into account the value of well known two-center integrals in the theory of molecules,[29] we have

$$
I_{ee}(r)=2E_b\exp\left(-\frac{2r}{a_x}\right)\frac{a_x}{r}\left[1+\frac{r}{a_x}+\frac{1}{3}\left(\frac{r}{a_x}\right)^2\right]^2 \tag{6}
$$

$$
I_{eh}(r)=2E_b\exp\left(-\frac{2r}{a_x}\right)\left(1+\frac{r}{a_x}\right)\left[1+\frac{r}{a_x}+\frac{1}{3}\left(\frac{r}{a_x}\right)^2\right], \tag{7}
$$

$$
\begin{aligned}
I_{hh}(r) &= 2E_b\left\{\left[\frac{5}{8}-\frac{23}{20}\frac{r}{a_x}-\frac{3}{5}\left(\frac{r}{a_x}\right)^2-\frac{1}{15}\left(\frac{r}{a_x}\right)^3\right]\exp\left(-2\frac{r}{a_x}\right)\right.\\
&+\frac{6}{5}\frac{a_x}{r}\left(\gamma+\ln\frac{r}{a_x}\right)\left[1+\frac{r}{a_x}+\frac{1}{3}\left(\frac{r}{a_x}\right)^2\right]^2\exp\left(-2\frac{r}{a_x}\right)\\
&+\frac{6}{5}\frac{a_x}{r}\left[1-\frac{r}{a_x}+\frac{1}{3}\left(\frac{r}{a_x}\right)^2\right]^2\exp\left(2\frac{r}{a_x}\right)\, Ei\left(-4\frac{r}{a_x}\right)\\
&\left.-\frac{12}{5}\frac{a_x}{r}\left[1-\frac{r}{a_x}+\frac{1}{3}\left(\frac{r}{a_x}\right)^2\right]\left[1+\frac{r}{a_x}+\frac{1}{3}\left(\frac{r}{a_x}\right)^2\right]Ei\left(-2\frac{r}{a_x}\right)\right\},
\end{aligned}
\tag{8}
$$

where $\mathrm{Ei}(z)=-\int\limits_{-z}^{\infty}\exp(-y)/y\,dy$ is the exponent integral and $\gamma\simeq 0.577$ – the Euler's constant.

To calculate approximately the inner integrals in equation (4), we expand the exponent in their integrand into series in powers of $\beta$. For the electron-electron and electron-hole exchange terms, integrals over $\mathbf{r}_1$ and $\mathbf{r}_2$ are just products of the two-center integral

$$
\int d^3r_1\exp[i\beta\mathbf{q}\mathbf{r}_1] f(r_1)\, f(|\mathbf{r}_1+\mathbf{r}|), \tag{9}
$$

or

$$
\int d^3r_1\exp[i\beta\mathbf{q}\mathbf{r}_1] f(r_1)\, f(|\mathbf{r}_1+\mathbf{r}|)\frac{a_x}{|\mathbf{r}_1+\mathbf{r}|}, \tag{10}
$$

on the complex conjugate of integral (9). Expanding the exponent in terms of spherical harmonics and going then to the elliptical variables $\lambda,\mu$ and $\varphi$, we give integrals (9) and (10) the following

form

$$\int d^3 r_1 \exp[i\beta \mathbf{q}\mathbf{r}_1] f(r_1)\, f(|\mathbf{r}_1+\mathbf{r}|) = \frac{1}{4}\left(\frac{r}{a_x}\right)^3 \exp\left(-i\frac{\beta}{2}\mathbf{q}\mathbf{r}\right)\sum_{n=0}^{\infty}(-1)^n(4n+1)P_{2n}(0)^2$$

$$\times \int_{-1}^{1} d\mu \int_{1}^{\infty} d\lambda \left(\lambda^2-\mu^2\right)\exp\left(-\frac{r}{a_x}\lambda - i\frac{\beta \mathbf{q}\mathbf{r}}{2}\lambda\mu\right)\; j_{2n}\left[\beta\sqrt{q^2r^2-(\mathbf{q}\mathbf{r})^2}\sqrt{(\lambda^2-1)(1-\mu^2)}/2\right], \quad (11)$$

and

$$\int d^3 r_1 \exp[i\beta \mathbf{q}\mathbf{r}_1] f(r_1)\, f(|\mathbf{r}_1+\mathbf{r}|)\frac{a_x}{|\mathbf{r}_1+\mathbf{r}|} = \frac{1}{2}\left(\frac{r}{a_x}\right)^2 \exp\left(-i\frac{\beta}{2}\mathbf{q}\mathbf{r}\right)\sum_{n=0}^{\infty}(-1)^n(4n+1)P_{2n}(0)^2$$

$$\times \int_{-1}^{1} d\mu \int_{1}^{\infty} dx \left(\lambda+\mu\right)\exp\left(-\frac{r}{a_x}\lambda - i\frac{\beta \mathbf{q}\mathbf{r}}{2}\lambda\mu\right)\; j_{2n}\left[\beta\sqrt{q^2r^2-(\mathbf{q}\mathbf{r})^2}\sqrt{(\lambda^2-1)(1-\mu^2)}/2\right], \quad (12)$$

where $P_{2n}(0)$ are Legendre polynomials at zero and $j_{2n}(x)$ are spherical Bessel functions. Truncating the sum over $n$ in the right hand side (rhs) of equations (11) and (12) at the term proportional to $\beta^3$ and then calculating the obtained integrals, we get approximate results for integrals (9) and (10). As a result,

$$\int d^3 r_1 \int d^3 r_2 \exp[i\beta \mathbf{q}(\mathbf{r}_1-\mathbf{r}_1)] f(r_1)\, f(|\mathbf{r}_1+\mathbf{r}|) f(r_2)\, f(|\mathbf{r}_2+\mathbf{r}|)\left[-\frac{a_x}{r}+2\frac{a_x}{|\mathbf{r}_1+\mathbf{r}|}\right]$$

$$= -I_{ee}(r) + 2I_{eh}(r) - i\frac{\beta}{6}2I_{eh}(r)\mathbf{q}\mathbf{r} - \beta^2\left[\mathcal{U}_{2a}(r)\,(\mathbf{q}\mathbf{r})^2 + \mathcal{U}_{2b}(r)(qa_x)^2\right]$$

$$+ i\frac{\beta^3}{60}\left[I_{eh}(r)\,(\mathbf{q}\mathbf{r})^3 + \mathcal{U}_3(r)\mathbf{q}\mathbf{r}(qa_x)^2\right] + O\left(\beta q a_x\right)^4, \quad (13)$$

where

$$\mathcal{U}_{2a}(r) = \frac{2}{15}\,I_{eh}(r) - \frac{1}{20}\,I_{ee}(r) \quad (14)$$

$$\mathcal{U}_{2b}(r) = 2E_b\exp\left(-\frac{2r}{a_x}\right)\left\{2\left[\frac{3}{4}+\frac{3}{2}\frac{r}{a_x}+\frac{67}{60}\left(\frac{r}{a_x}\right)^2+\frac{2}{5}\left(\frac{r}{a_x}\right)^3+\frac{11}{180}\left(\frac{r}{a_x}\right)^4\right]\right.$$

$$\left. -\left[1+\frac{r}{a_x}+\frac{1}{3}\left(\frac{r}{a_x}\right)^2\right]\left[1+\frac{r}{a_x}+\frac{2}{5}\left(\frac{r}{a_x}\right)^2+\frac{1}{15}\left(\frac{r}{a_x}\right)^3\right]\right\}, \quad (15)$$

$$\mathcal{U}_3(r) = 2E_b\exp\left(-\frac{2r}{a_x}\right)\left[13+26\frac{r}{a_x}+19\left(\frac{r}{a_x}\right)^2+\frac{20}{3}\left(\frac{r}{a_x}\right)^3+\left(\frac{r}{a_x}\right)^4\right]. \quad (16)$$

It is more complicated with the inner integral of the last term in braces in equation (4), which in the case $\beta = 0$ gives the two-electron two-center integral $I_{hh}$. We first expand the exponent in series in powers of $\beta$ retaining the first four terms. From the symmetry of the considered integral

in relation to $\mathbf{r}_1$ and $\mathbf{r}_2$ we can see, that the integrals going with $\beta$ and $\beta^3$ are zero. To calculate those ones which go with $\beta^2$,

$$\mathbf{K}^2 \int d^3r_1 d^3r_2 (\mathbf{r}_1 - \mathbf{r}_2)^2 f(|\mathbf{r}_1 + \mathbf{r}/2|)\, f(|\mathbf{r}_1 - \mathbf{r}/2|) f(|\mathbf{r}_2 + \mathbf{r}/2|)\, f(|\mathbf{r}_2 - \mathbf{r}/2|) \frac{a_x}{|\mathbf{r}_1 - \mathbf{r}_2|},$$

($\mathbf{K} \equiv \mathbf{q} + \mathbf{k}$) we go to the elliptical coordinates using the Neumann expansion for the inverse distance,

$$\frac{1}{|\mathbf{r}_1 - \mathbf{r}_2|} = \frac{2}{r} \sum_{\tau=0}^{\infty} \sum_{\nu=0}^{\tau} D_{\tau\nu} Q_\tau^\nu(\lambda_>) P_\tau^\nu(\lambda_<) P_\tau^\nu(\mu_1) P_\tau^\nu(\mu_2) \cos\left[\nu(\varphi_1 - \varphi_2)\right], \tag{17}$$

where $P_\tau^\nu(\mu)$ are associated Legendre polynomials, $P_\tau^\nu(\lambda_<)$ and $Q_\tau^\nu(\lambda_>)$ – Legendre functions with $\lambda_>$ ($\lambda_<$) the larger (smaller) of $\lambda_1$ and $\lambda_2$, $D_{\tau 0} = (2\tau + 1)$ and

$$D_{\tau\nu} = (-1)^\nu 2(2\tau + 1) \left[\frac{(\tau - \nu)!}{(\tau + \nu)!}\right]^2, \ \nu \geq 1.$$

Upon integration over $\varphi_1$ and $\varphi_2$, there remains one term from the sum over $\nu$ in rhs of equation (17). Further, integration over $\mu_1$ and $\mu_2$ leaves a finite number of terms from the sum over $\tau$,which are just twofold integrals over $\lambda_1$ and $\lambda_1$ from products of Legendre functions on exponents and powers functions, which are ready in closed analyticalforms. Taking the corresponding integrals, we get

$$\begin{aligned} &\int d^3r_1 d^3r_2 \exp[i\beta(\mathbf{k} + \mathbf{q})(\mathbf{r}_1 - \mathbf{r}_2)]\, f(|\mathbf{r}_1 + \mathbf{r}/2|)\, f(|\mathbf{r}_1 - \mathbf{r}/2|) f(|\mathbf{r}_2 + \mathbf{r}/2|)\, f(|\mathbf{r}_2 - \mathbf{r}/2|) \frac{a_x}{|\mathbf{r}_1 - \mathbf{r}_2|} \\ = \ & \mathcal{U}_{hh}(r) - \beta^2 \left[\mathcal{U}_{2c}(r)\, (\mathbf{kr} + \mathbf{qr})^2 + \mathcal{U}_{2d}(r)\, (|\mathbf{k} + \mathbf{q}| a_x)^2\right] + O\,(\beta q a_x)^4 \end{aligned} \tag{18}$$

with

$$\begin{aligned} \mathcal{U}_{2c}(r) \ = \ & 2E_b \left(\frac{a_x}{r}\right)^5 \Bigg\{ -\left(\frac{r}{a_x}\right)^2 \Bigg[\frac{738}{7} + \frac{492}{7}\frac{r}{a_x} + \frac{243}{7}\left(\frac{r}{a_x}\right)^2 + \frac{1391}{140}\left(\frac{r}{a_x}\right)^3 \\ & + \frac{83}{42}\left(\frac{r}{a_x}\right)^4 + \frac{5}{21}\left(\frac{r}{a_x}\right)^5 + \frac{1}{70}\left(\frac{r}{a_x}\right)^6\Bigg] \exp\left(-\frac{2r}{a_x}\right) \\ & + \Bigg[\frac{369}{7} + \frac{738}{7}\frac{r}{a_x} + \frac{675}{7}\left(\frac{r}{a_x}\right)^2 + \frac{366}{7}\left(\frac{r}{a_x}\right)^3 + \frac{654}{35}\left(\frac{r}{a_x}\right)^4 \\ & + \frac{159}{35}\left(\frac{r}{a_x}\right)^5 + \frac{5}{7}\left(\frac{r}{a_x}\right)^6 + \frac{2}{35}\left(\frac{r}{a_x}\right)^7\Bigg] \left(\gamma + \ln\frac{r}{a_x}\right) \exp\left(-\frac{2r}{a_x}\right) \\ & + \Bigg[\frac{369}{7} - \frac{738}{7}\frac{r}{a_x} + \frac{675}{7}\left(\frac{r}{a_x}\right)^2 - \frac{366}{7}\left(\frac{r}{a_x}\right)^3 + \frac{654}{35}\left(\frac{r}{a_x}\right)^4 \\ & - \frac{159}{35}\left(\frac{r}{a_x}\right)^5 + \frac{5}{7}\left(\frac{r}{a_x}\right)^6 - \frac{2}{35}\left(\frac{r}{a_x}\right)^7\Bigg] \exp\left(\frac{2r}{a_x}\right) Ei\left(-4\frac{r}{a_x}\right) \\ & - 2\left[\frac{369}{7} - 9\left(\frac{r}{a_x}\right)^2 + \frac{54}{35}\left(\frac{r}{a_x}\right)^4 + \frac{1}{7}\left(\frac{r}{a_x}\right)^6\right] Ei\left(-2\frac{r}{a_x}\right)\Bigg\}, \end{aligned} \tag{19}$$

and

$$
\begin{aligned}
\mathcal{U}_{2d}(r) \;=\;& 2E_b\left(\frac{a_x}{r}\right)^3\left\{\left(\frac{r}{a_x}\right)^2\left[\frac{246}{7}+\frac{15499}{672}\frac{r}{a_x}+\frac{3931}{336}\left(\frac{r}{a_x}\right)^2\right.\right.\\
&\left.+\frac{391}{120}\left(\frac{r}{a_x}\right)^3+\frac{61}{105}\left(\frac{r}{a_x}\right)^4+\frac{1}{21}\left(\frac{r}{a_x}\right)^5\right]\exp\left(-\frac{2r}{a_x}\right)\\
&-\left[\frac{123}{7}+\frac{246}{7}\frac{r}{a_x}+\frac{228}{7}\left(\frac{r}{a_x}\right)^2+\frac{128}{7}\left(\frac{r}{a_x}\right)^3+\frac{244}{35}\left(\frac{r}{a_x}\right)^4\right.\\
&\left.+\frac{13}{7}\left(\frac{r}{a_x}\right)^5+\frac{34}{105}\left(\frac{r}{a_x}\right)^6+\frac{1}{35}\left(\frac{r}{a_x}\right)^7\right]\left(\gamma+\ln\frac{r}{a_x}\right)\exp\left(-\frac{2r}{a_x}\right)\\
&-\left[\frac{123}{7}-\frac{246}{7}\frac{r}{a_x}+\frac{228}{7}\left(\frac{r}{a_x}\right)^2-\frac{128}{7}\left(\frac{r}{a_x}\right)^3+\frac{244}{35}\left(\frac{r}{a_x}\right)^4\right.\\
&\left.-\frac{13}{7}\left(\frac{r}{a_x}\right)^5+\frac{34}{105}\left(\frac{r}{a_x}\right)^6-\frac{1}{35}\left(\frac{r}{a_x}\right)^7\right]\exp\left(\frac{2r}{a_x}\right)Ei\left(-4\frac{r}{a_x}\right)\\
&\left.+2\left[\frac{123}{7}-\frac{18}{7}\left(\frac{r}{a_x}\right)^2+\frac{2}{5}\left(\frac{r}{a_x}\right)^4+\frac{8}{105}\left(\frac{r}{a_x}\right)^6\right]Ei\left(-2\frac{r}{a_x}\right)\right\}. \qquad (20)
\end{aligned}
$$

Thus we have

$$
\begin{aligned}
&\frac{1}{V}\sum_{\mathbf{q}}U^{ex}(2\mathbf{s},\mathbf{q})\psi(\mathbf{s}+\mathbf{q})\approx\int d^3r\exp[2i\alpha\mathbf{s}\mathbf{r}]\int d^3r'\exp[-i\mathbf{s}\mathbf{r}']\phi(r')\\
&\times\frac{1}{V}\sum_{\mathbf{q}}\exp[i\mathbf{q}(\alpha\mathbf{r}-\mathbf{r}')]\left\{-I_{ee}(r)+2I_{eh}(r)-i\frac{\beta}{6}2I_{eh}(r)\mathbf{q}\mathbf{r}\right.\\
&\left.-\beta^2\left[\mathcal{U}_{2a}(r)\,(\mathbf{q}\mathbf{r})^2+\mathcal{U}_{2b}(r)(qa_x)^2\right]+i\frac{\beta^3}{60}\left[I_{eh}(r)\,(\mathbf{q}\mathbf{r})^3+\mathcal{U}_3(r)(qa_x)^2\,\mathbf{q}\mathbf{r}\right]\right\}\\
&-\int d^3r\int d^3r'\exp[-i\mathbf{s}\mathbf{r}']\phi(r')\frac{1}{V}\sum_{\mathbf{q}}\exp[-i\mathbf{q}(\alpha\mathbf{r}+\mathbf{r}')]\\
&\times\left\{I_{hh}(r)-\beta^2\left[\mathcal{U}_{2c}(r)\,(2\mathbf{s}\mathbf{r}+\mathbf{q}\mathbf{r})^2+\mathcal{U}_{2d}(r)\,(|2\mathbf{s}+\mathbf{q}|a_x)^2\right]\right\}. \qquad (21)
\end{aligned}
$$

To proceed, we have to tackle the sums over $\mathbf{q}$ in nonlocal terms. First, we notice that

$$
\begin{aligned}
\frac{1}{V}\sum_{\mathbf{q}}\exp[i\mathbf{q}(\alpha\mathbf{r}-\mathbf{r}')]\mathbf{q}\mathbf{r} &= -i\frac{\partial}{\partial\alpha}\delta(\alpha\mathbf{r}-\mathbf{r}')\\
&= -i\,\frac{1}{\alpha}\mathbf{r}\nabla\delta(\alpha\mathbf{r}-\mathbf{r}'), \qquad (22)
\end{aligned}
$$

so the term proportional to $\beta$ in (21) is transformed as follows

$$
\begin{aligned}
&-\frac{i}{3}\int d^3r\,\exp[2i\alpha\mathbf{sr}]I_{eh}(r)\frac{\partial}{\partial\alpha}\int d^3r'\,\exp[-i\mathbf{sr}']\phi(r')\delta(\alpha\mathbf{r}-\mathbf{r}')\\
= &-\frac{1}{3}\int d^3r\,\exp[2i\alpha\mathbf{sr}]I_{eh}(r)\frac{\partial}{\partial\alpha}\left\{\exp[-i\alpha\mathbf{sr}]\phi(\alpha r)\right\}\\
= &-\frac{1}{3}\int d^3r\,\exp[i\alpha\mathbf{sr}]I_{eh}(r)\frac{\partial}{\partial\alpha}\phi(\alpha r)+\frac{\beta}{3}\int d^3r\,\underbrace{\exp[i\alpha\mathbf{sr}]\,i\mathbf{sr}}_{\frac{1}{\alpha}\mathbf{r}\nabla\exp[i\alpha\mathbf{sr}]}\,I_{eh}(r)\phi(\alpha r)\\
= &-\frac{1}{3}\int d^3r\,\exp[i\alpha\mathbf{sr}]I_{eh}(r)r\phi'-\frac{\beta}{3\alpha}\int d^3r\,\exp[i\alpha\mathbf{sr}]\,\nabla\left[I_{eh}(r)\phi(\alpha r)\mathbf{r}\right],
\end{aligned}
$$

so

$$
\begin{aligned}
&-i\frac{\beta}{3}\int d^3r\,\exp[2i\alpha\mathbf{sr}]I_{eh}(r)\frac{\partial}{\partial\alpha}\int d^3r'\,\exp[-i\mathbf{sr}']\phi(r')\delta(\alpha\mathbf{r}-\mathbf{r}')\\
= &-\frac{\beta}{3}\int d^3r\,\exp[2i\alpha\mathbf{sr}]I_{eh}(r)\frac{\partial}{\partial\alpha}\left\{\exp[-i\alpha\mathbf{sr}]\phi(\alpha r)\right\}\\
= &-\frac{\beta}{3}\int d^3r\,\exp[i\alpha\mathbf{sr}]I_{eh}(r)\frac{\partial}{\partial\alpha}\phi(\alpha r)+\frac{\beta}{3}\int d^3r\,\underbrace{\exp[i\alpha\mathbf{sr}]\,i\mathbf{sr}}_{\frac{1}{\alpha}\mathbf{r}\nabla\exp[i\alpha\mathbf{sr}]}\,I_{eh}(r)\phi(\alpha r)\\
= &-\frac{\beta}{3}\int d^3r\,\exp[i\alpha\mathbf{sr}]I_{eh}(r)r\phi'-\frac{\beta}{3\alpha}\int d^3r\,\exp[i\alpha\mathbf{sr}]\,\nabla\left[I_{eh}(r)\phi(\alpha r)\mathbf{r}\right],
\end{aligned}
$$

where the last term on the last line is obtained by integration by parts taking into account the fact, that $I_{eh}(r)\propto\exp[-2r/a_x]$ approaches zero at infinity. As a result, the first nonlocal term in the rhs of equation (21) yields

$$
-\frac{\beta}{3}\int d^3r\,\exp[i\alpha\mathbf{sr}]\left\{\frac{1}{\alpha}\left[I_{eh}(r)+r\frac{d}{dr}I_{eh}(r)\right]\phi(\alpha r)+2I_{eh}(r)r\,\phi'(\alpha r)\right\}. \tag{23}
$$

In the same way as the last result has been obtained, we write

$$
\begin{aligned}
\frac{1}{V}\sum_{\mathbf{q}}\exp[i\mathbf{q}(\alpha\mathbf{r}-\mathbf{r}')]\,(\mathbf{qr})^2 &= -\frac{\partial^2}{\partial\alpha^2}\delta(\alpha\mathbf{r}-\mathbf{r}')\\
\frac{1}{V}\sum_{\mathbf{q}}\exp[i\mathbf{q}(\alpha\mathbf{r}-\mathbf{r}')]\,(qa_x)^2 &= -\left(a_x\frac{\nabla}{\alpha}\right)^2\delta(\alpha\mathbf{r}-\mathbf{r}'),
\end{aligned}
$$

to start transformation of the terms going with $\beta^2$ in the rhs of equation (21). After repeative elementary operations of differentiation and integration in parts, we gain

$$
\begin{aligned}
&\int d^3r\,\mathcal{U}(r)\exp[2i\alpha\mathbf{sr}]\int d^3r'\,\exp[-i\mathbf{sr}']\phi(r')\,\frac{1}{V}\sum_{\mathbf{q}}\exp[i\mathbf{q}(\alpha\mathbf{r}-\mathbf{r}')]\,(\mathbf{qr})^2\\
= &\int d^3r\,\mathcal{U}(r)\int d^3r'\,\exp[-i\mathbf{sr}']\phi(r')\mathcal{U}(r)\frac{1}{V}\sum_{\mathbf{q}}\exp[-i\mathbf{q}(\alpha\mathbf{r}+\mathbf{r}')]\,(2\mathbf{sr}+\mathbf{qr})^2\\
= &\int d^3r\,\exp[i\alpha\mathbf{sr}]\,\mathcal{U}(r)\left\{-r^2\phi''(\alpha r)+2i\,\mathbf{sr}\,r\phi'(\alpha r)+(\mathbf{sr})^2\,\phi(\alpha r)\right\},
\end{aligned}
$$

$$\int d^3r\, \mathcal{U}(r) \exp[2i\alpha\mathbf{sr}] \int d^3r' \exp[-i\mathbf{sr}']\phi(r')\, \frac{1}{V} \sum_{\mathbf{q}} \exp[i\mathbf{q}(\alpha\mathbf{r} - \mathbf{r}')]\, (qa_x)^2$$

$$= \int d^3r\, \mathcal{U}(r) \int d^3r' \exp[-i\mathbf{sr}']\phi(r') \frac{1}{V} \sum_{\mathbf{q}} \exp[-i\mathbf{q}(\alpha\mathbf{r} + \mathbf{r}')]\, (|\mathbf{2s} + \mathbf{q}|a_x)^2$$

$$= \int d^3r\, \mathcal{U}(r) \exp[i\alpha\mathbf{sr}] \left\{ -\left(a_x\frac{\nabla}{\alpha}\right)^2 \phi(\alpha r) + 2ia_x^2 \left(\mathbf{s}\frac{\nabla}{\alpha}\right) \phi(\alpha r) + (sa_x)^2\, \phi(\alpha r) \right\}.$$

Making further transformations of the same type with the terms contaning $\mathbf{s}$ and $\mathbf{r}$, we get the second nonlocal term in the form

$$-\beta^2 \int d^3r\, \left\{ \mathcal{U}_{2A}(r) \left[ -\frac{\partial^2}{\partial\alpha^2}\phi(\alpha r) + \left(2\frac{\partial}{\partial\alpha}\phi(\alpha r) + \frac{\phi(\alpha r)}{\alpha}\right)\left(\mathbf{r}\frac{\nabla}{\alpha}\right) - \phi(\alpha r)\left(\mathbf{r}\frac{\nabla}{\alpha}\right)^2 \right] \right.$$
$$\left. + a_x^2\, \mathcal{U}_{2B}(r) \left[ -\left(\frac{\nabla}{\alpha}\right)^2 \phi(\alpha r) + 2\frac{\nabla}{\alpha}\phi(\alpha r)\frac{\nabla}{\alpha} - \phi(\alpha r)\left(\mathbf{r}\frac{\nabla}{\alpha}\right)^2 \right] \right\} \exp[i\alpha\mathbf{sr}]$$

with $\mathcal{U}_{2A}(r) = \mathcal{U}_{2a}(r) + \mathcal{U}_{2c}(r)$ and $\mathcal{U}_{2B}(r) = \mathcal{U}_{2b}(r) + \mathcal{U}_{2d}(r)$. Performing integration of the terms containing $\nabla$ by parts, we recast the last expression to the final form

$$\beta^2 \int d^3r\, \exp[i\alpha\mathbf{sr}] \left\{ 4\left[r^2\mathcal{U}_{2A}(r) + a_x^2\,\mathcal{U}_{2B}(r)\right]\phi''(\alpha r) \right.$$
$$+ \frac{2}{\alpha}\left[3r\mathcal{U}_{2A}(r) + 4\frac{a_x^2}{r}\mathcal{U}_{2B}(r) + 2r^2\frac{d}{dr}\mathcal{U}_{2A}(r) + 2a_x^2\frac{d}{dr}\mathcal{U}_{2B}(r)\right]\phi'(\alpha r)$$
$$\left. + \frac{1}{\alpha^2}\left[2\mathcal{U}_{2A}(r) + 4r\frac{d}{dr}\mathcal{U}_{2A}(r) + 2\frac{a_x^2}{r}\frac{d}{dr}\mathcal{U}_{2B}(r) + r^2\frac{d^2}{dr^2}\mathcal{U}_{2A}(r) + a_x^2\frac{d^2}{dr^2}\mathcal{U}_{2B}(r)\right]\phi(\alpha r) \right\} \quad (24)$$

Finally, by writing

$$\frac{1}{V}\sum_{\mathbf{q}} \exp[i\mathbf{q}(\alpha\mathbf{r} - \mathbf{r}')]\, (\mathbf{qr})^2 = i\frac{\partial^3}{\partial\alpha^3}\delta(\alpha\mathbf{r} - \mathbf{r}')$$
$$\frac{1}{V}\sum_{\mathbf{q}} \exp[i\mathbf{q}(\alpha\mathbf{r} - \mathbf{r}')]\mathbf{qr}\, (qa_x)^2 = i\left(\mathbf{r}\frac{\nabla}{\alpha}\right)\left(a_x\frac{\nabla}{\alpha}\right)^2 \delta(\alpha\mathbf{r} - \mathbf{r}'),$$

and performing tedious elementary transformations, we obtain the terms going with $\beta^3$ in the rhs of equation (21) as follows

$$\frac{i}{60}\int d^3r\, I_{eh}(r) \exp[2i\alpha\mathbf{sr}] \int d^3r' \exp[-i\mathbf{sr}']\phi(r')\, \frac{1}{V}\sum_{\mathbf{q}} \exp[i\mathbf{q}(\alpha\mathbf{r} - \mathbf{r}')]\, (\mathbf{qr})^3$$
$$= -\frac{1}{60}\int d^3r \exp[i\alpha\mathbf{sr}] \left\{ 8r^3 I_{eh}(r)\phi'''(\alpha r)) + \frac{3r^2}{\alpha}\left[8I_{eh}(r) + 4r\frac{d}{dr}I_{eh}(r)\right]\phi''(\alpha r) \right.$$
$$+ \frac{r}{\alpha^2}\left[24I_{eh}(r) + 30r\frac{d}{dr}I_{eh}(r) + 6r^2\frac{d^2}{dr^2}I_{eh}(r)\right]\phi'(\alpha r)$$
$$\left. + \frac{1}{\alpha^3}\left[6I_{eh}(r) + 18r\frac{d}{dr}I_{eh}(r) + 9r^2\frac{d^2}{dr^2}I_{eh}(r) + r^3\frac{d^3}{dr^3}I_{eh}(r)\right]\phi(\alpha r) \right\}$$

and

$$
\begin{aligned}
&\frac{i}{60}\int d^3r\,\mathcal{U}_3(r)\exp[2i\alpha\mathbf{sr}]\int d^3r'\exp[-i\mathbf{sr}']\phi(r')\,\frac{1}{V}\sum_{\mathbf{q}}\exp[i\mathbf{q}(\alpha\mathbf{r}-\mathbf{r}')]\mathbf{qr}\,(qa_x)^2\\
=\; & -\frac{1}{60}\int d^3r\exp[i\alpha\mathbf{sr}]\left\{8r\mathcal{U}_3(r)\phi'''(\alpha r))+\frac{1}{\alpha}\left[28\mathcal{U}_3(r)+12r\frac{d}{dr}\mathcal{U}_3(r)\right]\phi''(\alpha r)\right.\\
&+\frac{1}{\alpha^2}\left[\frac{8}{r}\mathcal{U}_3(r)+24\frac{d}{dr}\mathcal{U}_3(r)+6r\,\frac{d^2}{dr^2}\mathcal{U}_3(r)\right]\phi'(\alpha r)\\
&\left.+\frac{1}{\alpha^3}\left[\frac{4}{r}\frac{d}{dr}\mathcal{U}_3(r)+5\,\frac{d^2}{dr^2}\mathcal{U}_3(r)+r\frac{d^3}{dr^3}\,\mathcal{U}_3(r)\right]\phi(\alpha r)\right\}. \qquad (25)
\end{aligned}
$$

With results (22) – (25), we have eventually

$$
\begin{aligned}
\frac{1}{2V}\sum_{\mathbf{q}}U^{ex}(2\mathbf{s},\mathbf{q})\psi(\mathbf{s}+\mathbf{q}) \;=\; & \int d^3r\exp[i\mathbf{sr}]\left\{A_0\,(r)+\beta\,A_1\,(r)\,\frac{d}{dr}\right.\\
&\left.+\beta^2A_2\,(r)\,\frac{d^2}{dr^2}+\beta^3A_3\,(r)\,\frac{d^3}{dr^3}+...\right\}\phi(r), \qquad (26)
\end{aligned}
$$

which is equation (8) in the article, where

$$
\begin{aligned}
A_0(r) \;=\; & \frac{1}{2\alpha^3}\left\{\mathcal{U}_0(\frac{r}{\alpha})-\frac{1}{3}\frac{\beta}{\alpha}\left[I_{eh}(\frac{r}{\alpha})+r\frac{d}{dr}\,I_{eh}(\frac{r}{\alpha})\right]\right.\\
&+\frac{\beta^2}{\alpha^2}\left[2\mathcal{U}_{2A}(\frac{r}{\alpha})+4\frac{r}{\alpha}\frac{d}{dr}\mathcal{U}_{2A}(\frac{r}{\alpha})+\frac{2\alpha}{r}a_x^2\frac{d}{dr}\mathcal{U}_{2B}(\frac{r}{\alpha})\right.\\
&\left.+\left(\frac{r}{\alpha}\right)^2\frac{d^2}{dr^2}\mathcal{U}_{2A}(\frac{r}{\alpha})+a_x^2\frac{d^2}{dr^2}\mathcal{U}_{2B}(\frac{r}{\alpha})\right]\\
&-\frac{1}{60}\frac{\beta^3}{\alpha^3}\left[6I_{eh}(\frac{r}{\alpha})+18\frac{r}{\alpha}\frac{d}{dr}I_{eh}(\frac{r}{\alpha})+9\left(\frac{r}{\alpha}\right)^2\frac{d^2}{dr^2}I_{eh}(\frac{r}{\alpha})\right.\\
&\left.\left.+\left(\frac{r}{\alpha}\right)^3\frac{d^3}{dr^3}I_{eh}(\frac{r}{\alpha})+\frac{4}{r}a_x^2\frac{d}{dr}\mathcal{U}_3(\frac{r}{\alpha})+5a_x^2\frac{d^2}{dr^2}\mathcal{U}_3(\frac{r}{\alpha})+\frac{r}{\alpha}\,a_x^2\frac{d^3}{dr^3}\mathcal{U}_3(\frac{r}{\alpha})\right]\right\}, \qquad (27)
\end{aligned}
$$

$$
\begin{aligned}
A_1(r) \;=\; & \frac{1}{2\alpha^3}\left\{-\frac{2}{3}\frac{r}{\alpha}\,I_{eh}(\frac{r}{\alpha})+\frac{2\beta}{\alpha}\left[3\frac{r}{\alpha}\mathcal{U}_{2A}(\frac{r}{\alpha})+2\left(\frac{r}{\alpha}\right)^2\frac{d}{dr}\mathcal{U}_{2A}(\frac{r}{\alpha})\right.\right.\\
&\left.+\frac{4\alpha}{r}a_x^2\,\mathcal{U}_{2B}(\frac{r}{\alpha})+2a_x^2\frac{d}{dr}\,\mathcal{U}_{2B}(\frac{r}{\alpha})\right]\\
&-\frac{\beta^2}{\alpha^2}\left[\frac{2}{5}\frac{r}{\alpha}I_{eh}(\frac{r}{\alpha})+\frac{1}{2}\left(\frac{r}{\alpha}\right)^2\frac{d}{dr}\,I_{eh}(\frac{r}{\alpha})+\frac{1}{10}\left(\frac{r}{\alpha}\right)^3\frac{d^2}{dr^2}I_{eh}(\frac{r}{\alpha})\right.\\
&\left.\left.+\frac{\alpha}{15r}a_x^2\mathcal{U}_3(\frac{r}{\alpha})+\frac{1}{5}\,a_x^2\frac{d}{dr}\mathcal{U}_3(\frac{r}{\alpha})+\frac{1}{20}a_x^2\frac{r}{\alpha}\frac{d^2}{dr^2}\,\mathcal{U}_3(\frac{r}{\alpha})\right]\right\}, \qquad (28)
\end{aligned}
$$

$$A_2(r) = \frac{1}{2\alpha^3}\left\{4\left(\frac{r}{\alpha}\right)^2 \mathcal{U}_{2A}(\frac{r}{\alpha}) + 4a_x^2 \mathcal{U}_{2B}(\frac{r}{\alpha}) - \frac{\beta}{\alpha}\left[\frac{2}{5}\left(\frac{r}{\alpha}\right)^2 I_{eh}(\frac{r}{\alpha}) + \frac{1}{5}\left(\frac{r}{\alpha}\right)^3 \frac{d}{dr} I_{eh}(\frac{r}{\alpha}) + \frac{7}{30} a_x^2 \mathcal{U}_3(\frac{r}{\alpha}) + \frac{1}{10} r\, a_x^2 \frac{d}{dr}\mathcal{U}_3(\frac{r}{\alpha})\right]\right\} \tag{29}$$

$$A_3(r) = -\frac{1}{30\alpha^3}\frac{r}{\alpha}\left\{2\left(\frac{r}{\alpha}\right)^2 I_{eh}(\frac{r}{\alpha}) + a_x^2 \mathcal{U}_3(\frac{r}{\alpha})\right\}. \tag{30}$$

Now we can write equations for two bare channels in the real space,

$$-\frac{\hbar^2}{\mu_x}\nabla^2\phi_E(r) + \left[\mathcal{U}^d(r) + A_0(r) - E\right]\phi_E(r) + \beta A_1(r)\phi'_E(r) + \beta^2 A_2(r)\phi''_E(r) + \beta^3 A_3(r)\chi'''_E(r) = 0, \tag{31}$$

$$-\frac{\hbar^2}{\mu_x}\nabla^2\phi_E(r) + \left[\mathcal{U}^d(r) - A_0(r) + 2\Delta - E_0\right]\phi_b(r) - \beta A_1(r)\phi'_b(r) - \beta^2 A_2(r)\phi''_b(r) - \beta^3 A_3(r)\chi'''_b(r) = 0, \tag{32}$$

where $\phi_E(r)$ is the function of the s-wave background scattering at energy $E$ and $\phi_b(r)$ – that of the possible biexciton at energy $E_0$. By usual substitution $\phi = 4\pi\chi/r$ and putting then $x \equiv r/a_x$, we give equations (31) and (32) the following form

$$-\frac{\hbar^2}{\mu_x a_x^2}\chi''_E + \left[\mathcal{U}^d(x) + F_0(x) - E\right]\chi_E + \beta F_1(x)\chi'_E + \beta^2 F_2(x)\chi''_E + \beta^3 F_3(x)\chi'''_E = 0, \tag{33}$$

$$-\frac{\hbar^2}{\mu_x a_x^2}\chi''_b + \left[\mathcal{U}^d(x) - F_0(x) + 2\Delta - E_0\right]\chi_b - \beta F_1(x)\chi'_b - \beta^2 F_2(x)\chi''_b - \beta^3 F_3(x)\chi'''_b = 0. \tag{34}$$

Noting that $\hbar^2/a_x^2 = 2\mu_r E_b$ and $\mu_r/\mu_x = (1-\beta)\beta$, we see that equations (33) and (34) coincide with equations (8) and (9) in the article, respectively. Functions $F_0(x), F_1(x), F_2(x)$ and $F_3(x)$ are expressed in terms of $A_0(x), A_1(x), A_2(x)$ and $A_3(x)$ as follows

$$\begin{aligned}
F_0(x) &= A_0(x) - \frac{1}{x}A_1(x) + \frac{2}{x^2}A_2(x) - \frac{6}{x^3}A_3(x) \\
F_1(x) &= A_1(x) - \frac{2}{x}A_2(x) + \frac{6}{x^2}A_3(\frac{x}{\alpha}) \\
F_2(x) &= A_2(x) - \frac{3}{x}A_3(x) \\
F_3(x) &= A_3(x).
\end{aligned} \tag{35}$$
